# Supplementary material for: In-Context Unlearning: Language Models as Few Shot Unlearners
Source: arXiv:2310.07579 source file (2024-06-06)
Supplement: Supplementary file 1 [file section8_appendix.tex]

\section{Reproducibility} 
All experiments are run using Nvidia Tesla V100 GPUs.
We finetuned 60 models across two different model sizes and 4 different data sets; 30 models were finetuned using Bloom560M and another 30 models were finetuned using Bloom 1.1B.
On average, finetuning took approximately 1 hour per model, which makes for 60 GPU hours.
Regarding the main experiments, we conducted unlearning using both GA and ICUL.
First, for ICUL we ran inference across 3 context length configurations across 60 models and each run took 2 hours on average. 
This amount to 360 GPU hours.
Second, for GA, the situation was very similar.
Updating the models using GA across 3 learning rate configurations for all 60 models where each inference run took approximately 2 hours amounts to another 360 GPU hours.
Finally, we ran the additional sensitivity experiments on SST-2 using Bloom 1.1B. 
These experiments were conducted for 10 models, using 3 context length configurations and 3 sensitivity setups, where each inference run took approximately 1.5 hours, which makes for a total of 135 GPU hours.
In total, we used 855 GPU hours which approximately amounts to 36 GPU days.
Note that these numbers include run times to find competitive learning rates and context lengths.

%\section{Additional related works}
% Here we briefly discuss additional related works that study (supervised) in-context learning theoretically \citep{xie2021explanation,akyurek2022learning,von2023transformers,nagler2023statistical,zhang2023trained,mahankali2023one,panigrahi2023trainable,ahn2023transformers}. 
% Initially, \citet{garg2022can} empirically showed that linear transformers can learn simple function classes like linear regressors in-context. 
% Inspired by these observations, \citet{von2023transformers} puts forth a weight construction for trained transformers that implements a single step of gradient descent in a forward pass, which has subsequently been studied in more detail showing that the corresponding weight construction is globally optimal \citep{zhang2023trained,mahankali2023one,ahn2023transformers} and that gradient flow reaches this optimum \citep{zhang2023trained}. 

\section{Additional Experimental Results}
\label{app:additional_hyperparams}

%\subsection{Optimizing Hyperparameters}
%\label{app:optimizating_hyperparams}
Both \texttt{ICUL} and \texttt{GA} have each one crucial parameter, namely the context length and the learning rate.
Here we investigate the impact that these parameters have on unlearning success and model performance.

\textbf{Vary the context length on \texttt{ICUL}.}
For \texttt{ICUL}, changing the context length can significantly improve results in terms of unlearning success as seen in Figure \ref{fig:ubs1_context_length}.
In terms of model performance, the situation is more nuanced as can be seen from Figure \ref{fig:ubs1_performance_vary_context_length}.
While the context length has clear impact on forget points, test points seem to be impacted very little by the number of context examples.

\begin{figure}[htb]
\centering
\begin{subfigure}{\textwidth}
\centering
\includegraphics[width=\textwidth]{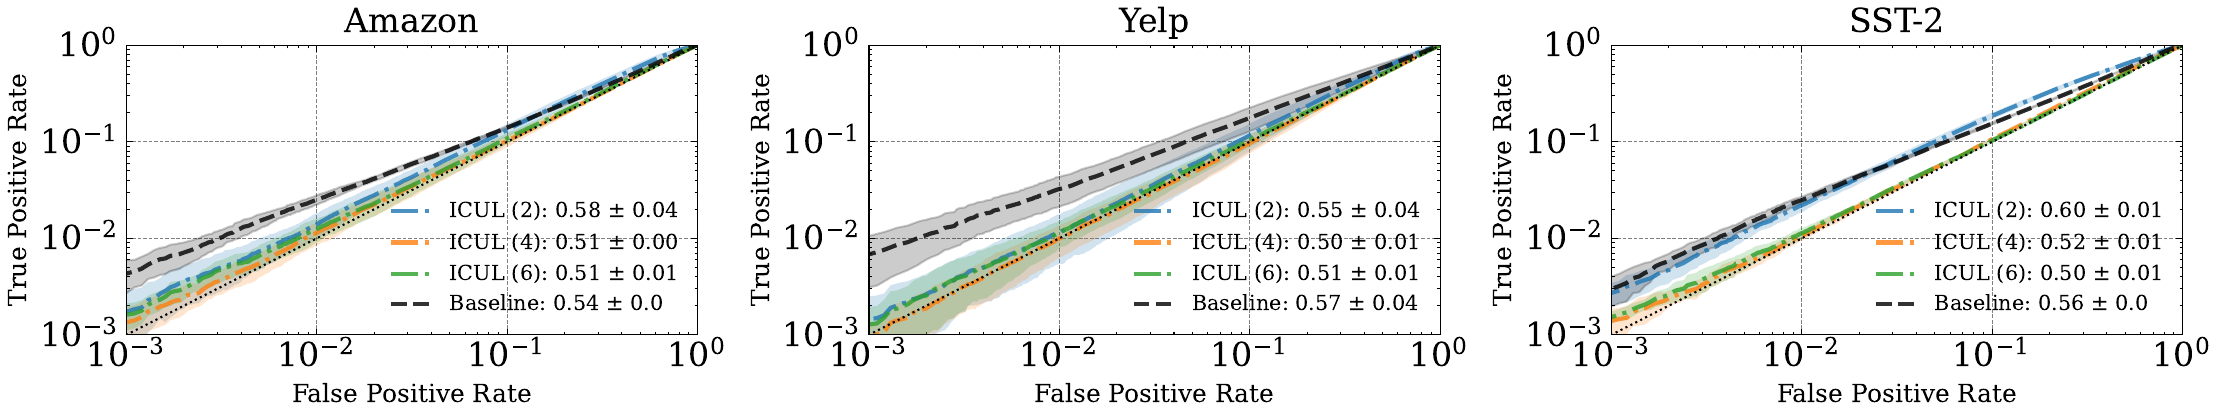}
\caption{Bloom (560M parameters)}
\label{fig:ubs1_vary_context_bloom560}
\end{subfigure}
\vfill
\begin{subfigure}{\textwidth}
\centering
\includegraphics[width=\textwidth]{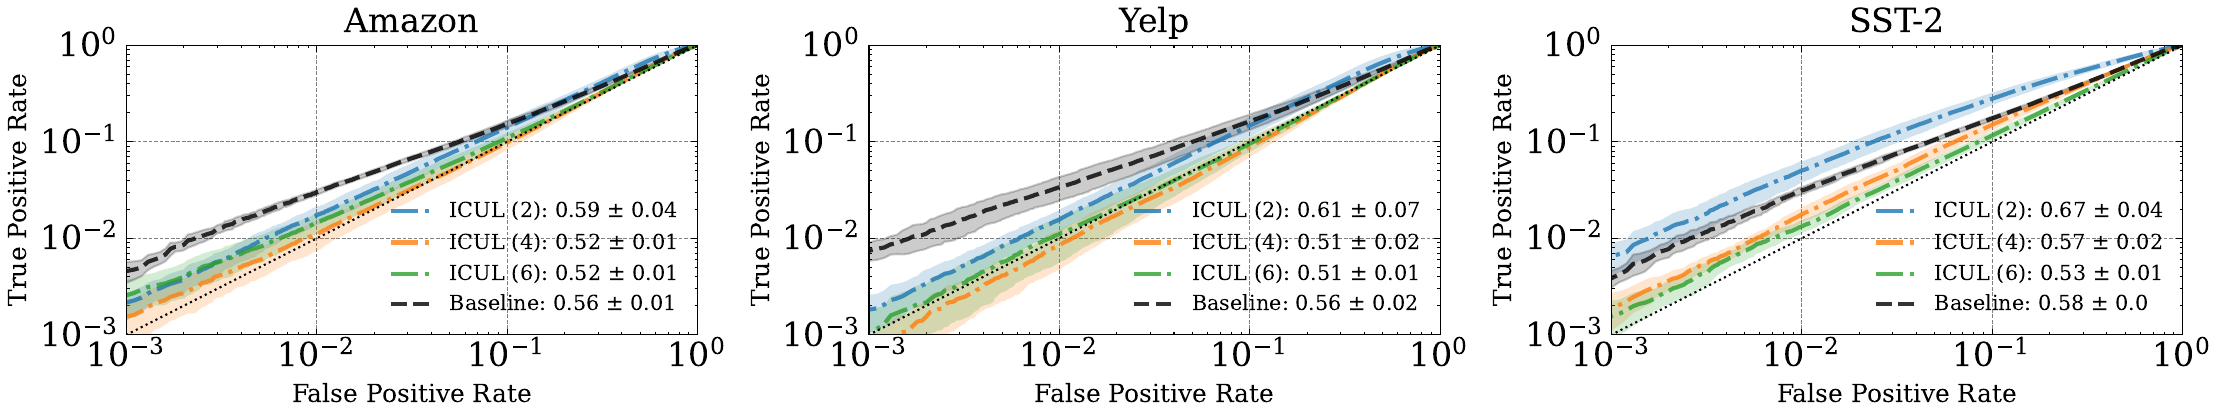}
\caption{Bloom (1.1B parameters)}
\label{fig:ubs1_vary_context_bloom1b1}
\end{subfigure}
\caption{\textbf{Varying context length for \texttt{ICUL}}. Same setup as in Figure \ref{fig:ubs1_unlearning_success}.
We plot the MI attack performance using log scaled ROC curves across different datasets and model sizes. 
The MI attacks were run against the updated models $\bar{f}$, which was updated using \texttt{ICUL}.
The closer to the diagonal, which amounts to the adversary randomly guessing whether a forget point is still part of the model or not, the better. 
The numbers in brackets denote the best parameters and the numbers after that show the AUC $\pm 1$ standard deviation across 10 evaluation runs. 
The black dashed line represents the baseline performance of not removing the point where the same attack is run on the model $f_{\theta(S)}$, as described in Section \ref{sec:eval_measures}. 
Shades indicate $\pm 1$ standard deviation across 10 evaluation runs.
}
\label{fig:ubs1_context_length}
\end{figure}

\begin{figure}[htb]
\centering
\begin{subfigure}{\textwidth}
\centering
\includegraphics[width=\textwidth]{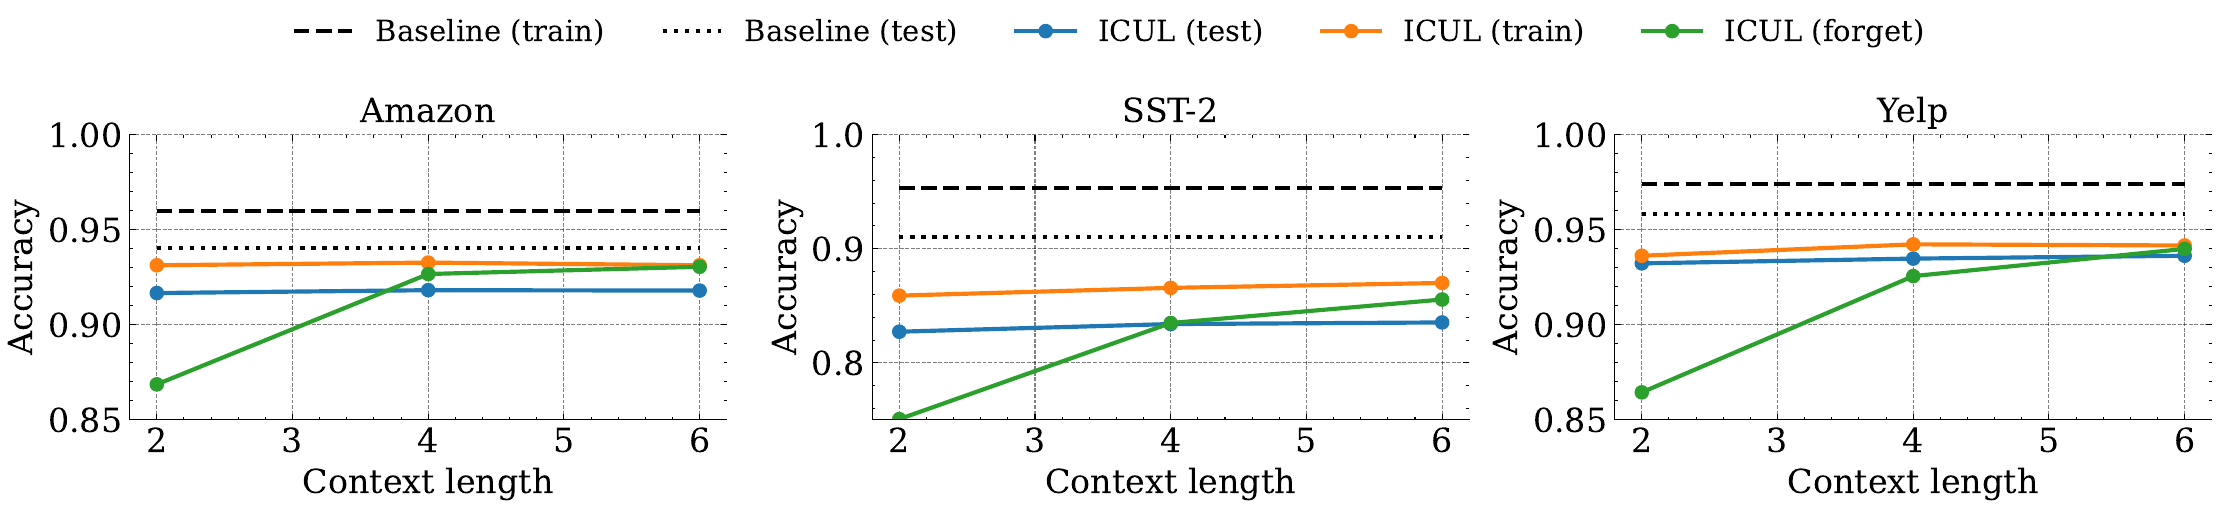}
\caption{Bloom (560M parameters)}
%\label{fig:ubs1_performance_vary_context_bloom560}
\end{subfigure}
\vfill
\begin{subfigure}{\textwidth}
\centering
\includegraphics[width=\textwidth]{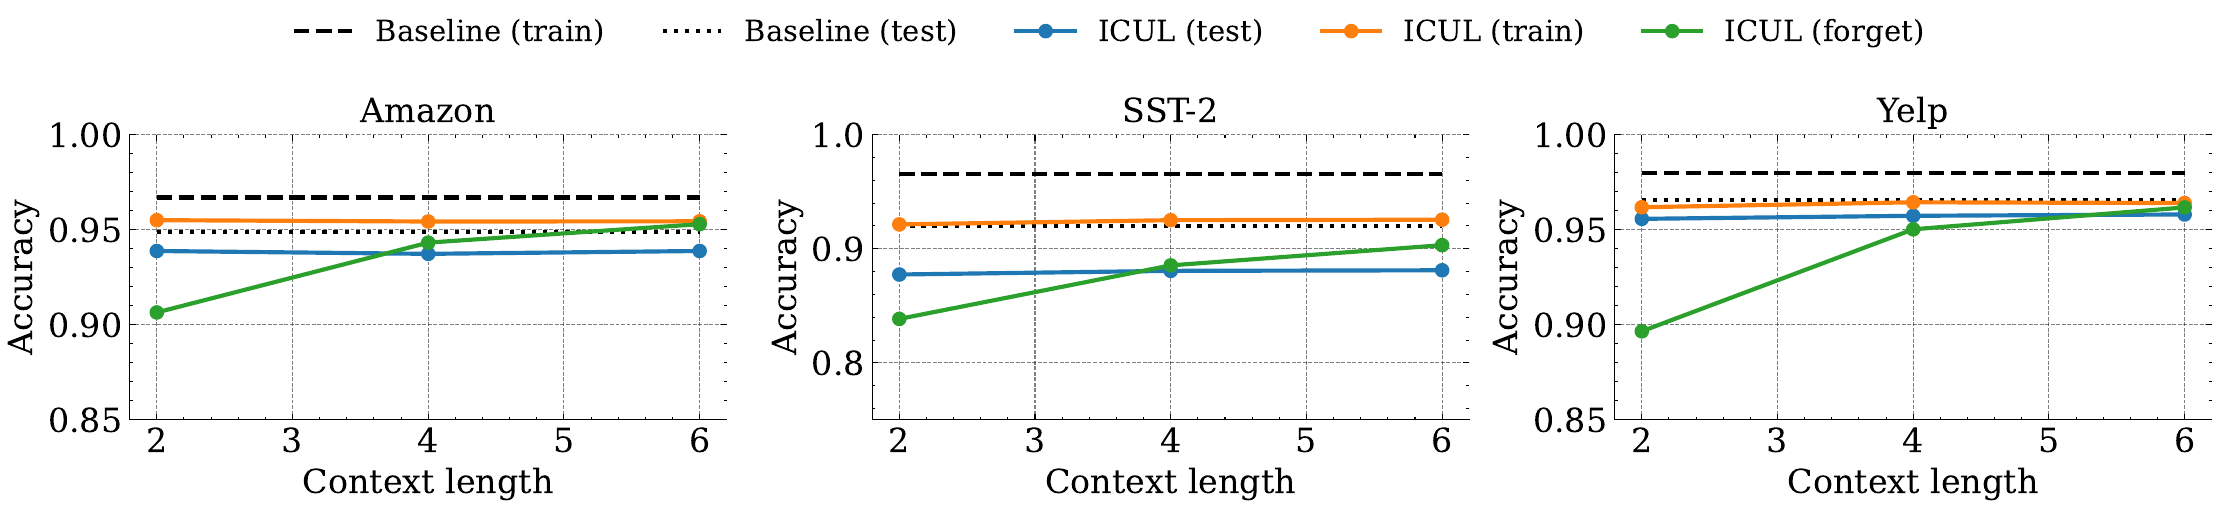}
\caption{Bloom (1.1B parameters)}
%\label{fig:ubs1_performance_vary_context_bloom1b1}
\end{subfigure}
\caption{\textbf{Classification performance as we vary context length for \texttt{ICUL}}. We report classification accuracy on train, forget and test points across all data sets and model sizes.
For better readability, $\pm 1$ standard deviation was excluded from the figure.
}
\label{fig:ubs1_performance_vary_context_length}
\end{figure}

\textbf{Vary the learning rate on \texttt{GA}.}
For \texttt{GA}, changing the learning rate can dramatically improve results, where smaller learning rates usually significantly improve results in terms of unlearning success and model performance as shown in Figures \ref{fig:ubs1_vary_lr_info_leakage} and \ref{fig:ubs1_performance_vary_lr}.

\begin{figure}[htb]
\centering
\begin{subfigure}{\textwidth}
\centering
\includegraphics[width=\textwidth]{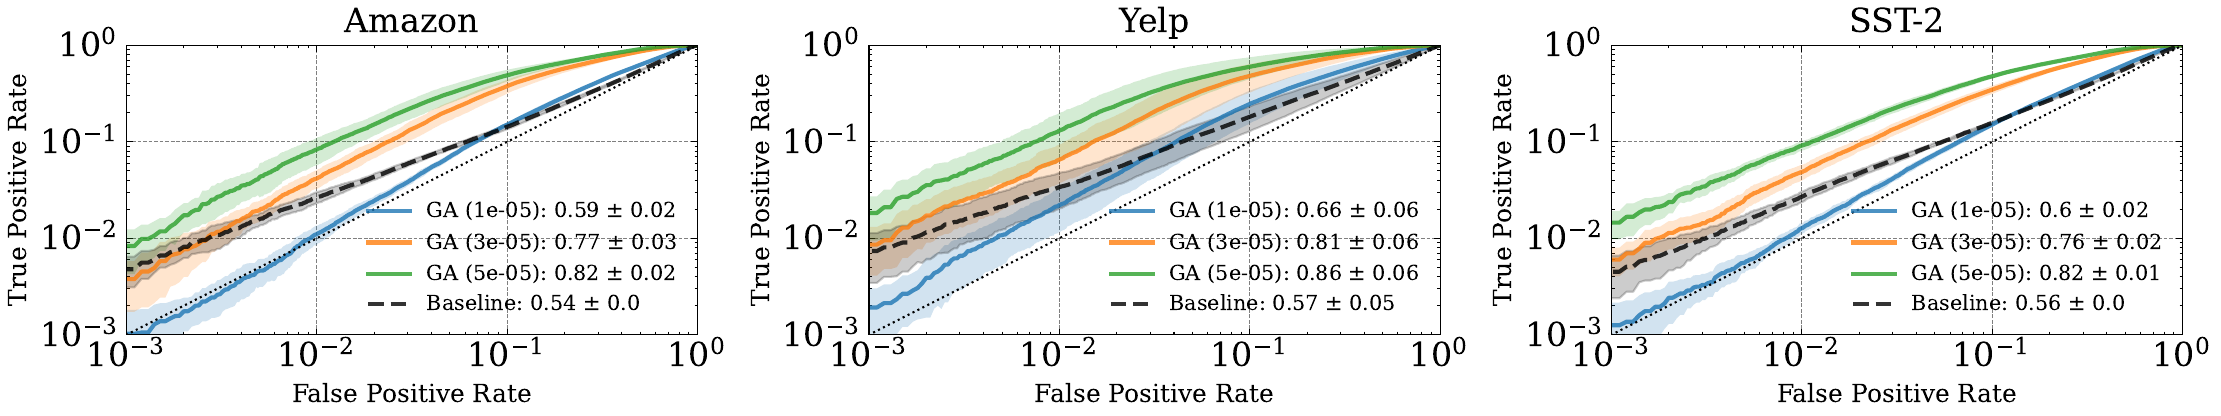}
\caption{Bloom (560M parameters)}
\label{fig:ubs1_vary_lr_bloom560_info_leakage}
\end{subfigure}
\vfill
\begin{subfigure}{\textwidth}
\centering
\includegraphics[width=\textwidth]{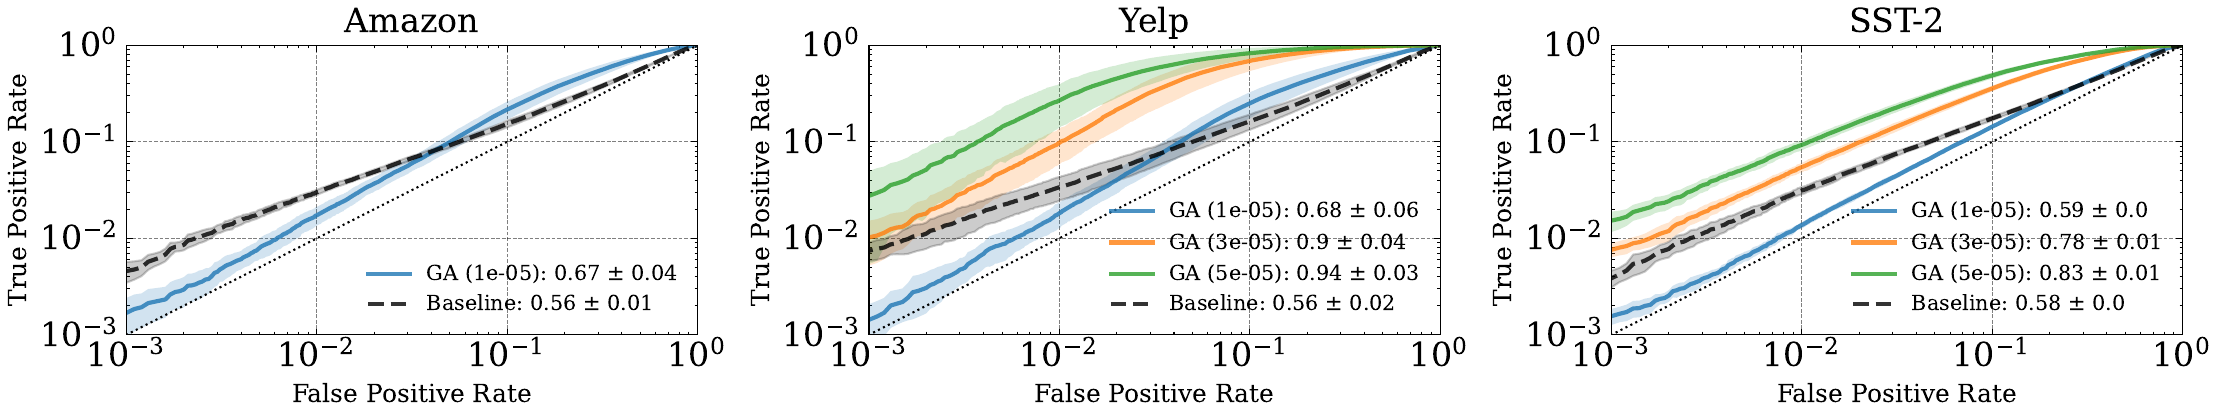}
\caption{Bloom (1.1B parameters)}
\label{fig:ubs1_vary_lr_bloom1b1_info_leakage}
\end{subfigure}
\caption{\textbf{Varying the learning rate for \texttt{GA}.} We plot the MI attack performance using log scaled ROC curves across different datasets and model sizes. 
The MI attacks were run against the updated models $\bar{f}$, which was updated using \texttt{GA}.
The closer to the diagonal, which amounts to the adversary randomly guessing whether a forget point is still part of the model or not, the better. 
The numbers in brackets denote the best parameters and the numbers after that show the AUC $\pm 1$ standard deviation across 10 evaluation runs. 
The black dashed line represents the baseline performance of not removing the point where the same attack is run on the model $f_{\theta(S)}$, as described in Section \ref{sec:eval_measures}. 
Shades indicate $\pm 1$ standard deviation across 10 evaluation runs.}
\label{fig:ubs1_vary_lr_info_leakage}
\end{figure}

\begin{figure}[htb]
\centering
\begin{subfigure}{\textwidth}
\centering
\includegraphics[width=\textwidth]{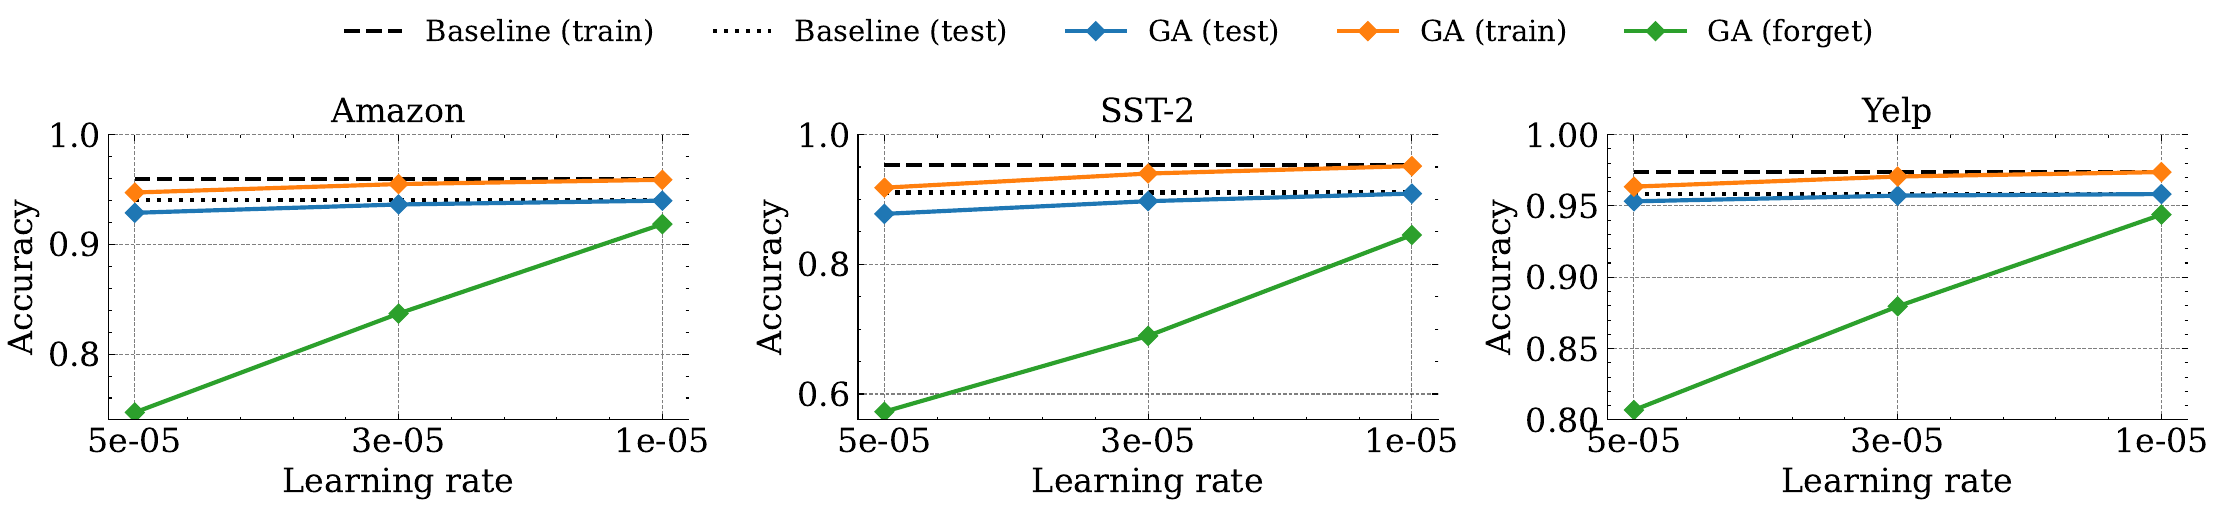}
\caption{Bloom (560M parameters)}
\label{fig:ubs1_performance_vary_lr_bloom560}
\end{subfigure}
\vfill
\begin{subfigure}{\textwidth}
\centering
\includegraphics[width=\textwidth]{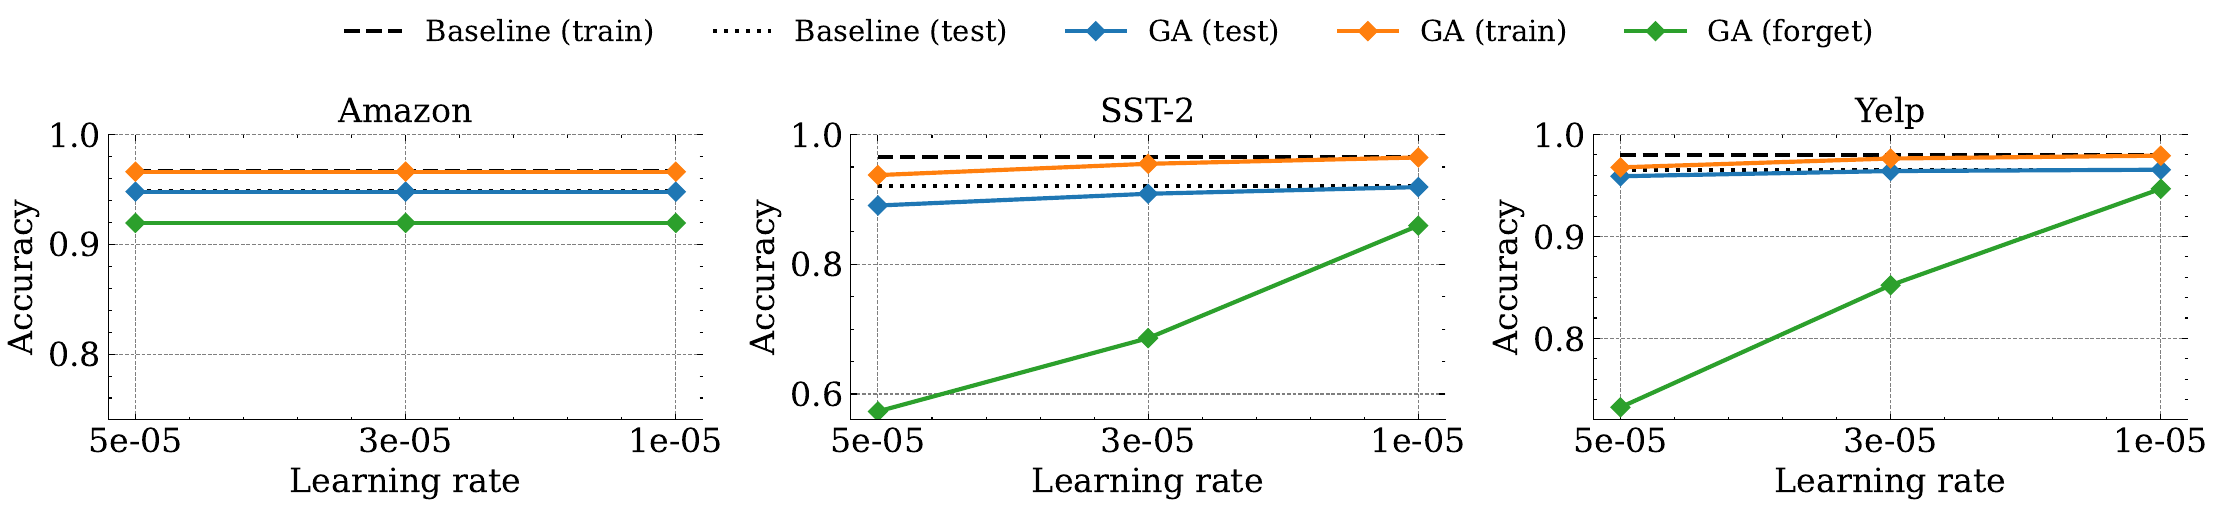}
\caption{Bloom (1.1B parameters)}
%\label{fig:ubs1_performance_vary_context_bloom1b1}
\end{subfigure}
\caption{\textbf{Classification performance as we vary the learning rate for \texttt{GA}}. We report classification accuracy on train, forget and test points across all data sets and model sizes.
For better readability, $\pm 1$ standard deviation was excluded from the figure.
}
\label{fig:ubs1_performance_vary_lr}
\end{figure}

\section{Details on the Machine Unlearning Evaluation}
\label{app:machine_unlearning}

% Taking inspiration from the Neyman-Pearson lemma \citep{neyman1933ix}, which asserts that the optimal hypothesis test at a predetermined false-positive rate involves thresholding the likelihood-ratio test $\Lambda$, we define the measure of unlearning success by comparing two distributions over models:
% \begin{equation}
% \Lambda = \frac{p\big(f_{\bar{\btheta}}\big)}{p\big(f_{\btheta(S \backslash S_f)}\big)}.
% \label{eq:optimal_lrt}
% \end{equation}
% In the first scenario, the model undergoes training using a randomly sampled training dataset $S$ containing the forget set $S_f$.
% Subsequently, the unlearning procedure $\mathcal{U}$ (approximately) removes the forget set $S_f$ from the trained model. 
% The second scenario involves the model being trained without the inclusion of the forget set $S_f$.
% Note that the likelihood ratio test in \eqref{eq:optimal_lrt} is not feasible as the distributions over models in the nominator and denominator are usually not analytically known.
% To make the situation more tractable, we
% instead define the distribution over losses on points $(\bx, y)$ for both models. 
% Then, we replace both distributions from  \eqref{eq:optimal_lrt} with the tractable test
% \begin{equation}
% \hat{\Lambda} = \frac{p\big(\ell\big( f_{\hat{\btheta}} (\bx),y\big)\big)}{p\big(\ell\big(f_{\btheta(S \backslash S_f)}(\bx), y\big)\big)},
% \label{eq:approx_lrt}
% \end{equation}
% where $\ell$ denotes an appropriate loss function.

\textbf{Operationalizing the Likelihood-ratio Audit.}
Operationalizing the likelihood ratio test from \eqref{eq:approx_lrt} requires access to the distribution of losses under the null and alternative hypotheses.
While analytical solutions are usually not available, we can readily get large samples from these two distributions.
In an ideal scenario, this entails that we would need to fit as many re-train models and unlearned models as possible for every forget set of interest.
Since this approach becomes computationally too burdensome, we use the following two-step approximation:

\textbf{Approximating the distributions under $H_0$ and $H_1$.} Here we adapt the sample splitting procedure first introduced by \citet{carlini2021membership} to forget sets with sizes $J$ greater than 1.
We train $K$ shadow models on random samples from the data distribution $\mathcal{D}$ so that a fraction $p$ of these models are trained on the forget set $S_f = \{(\bx_j, \mathbf{y}_j)\}_{j=1}^J$, and a fraction $(1-p)$ are not.
In particular, we train shadow models on $K=10$ subsets of $\mathcal{D}$ so that each forget set $S_f \in D$ appears in $K\cdot p$ subsets.
This approach has the advantage that the same $K$ shadow models can be used to estimate the likelihood-ratio test for all the forget sets.
Finally, we fit the parameters of two Gaussian distributions to the confidence scores of the retain models and the unlearned models on $S_f$. 
Across all experiments, we use $p=0.5$ and $J=1$.

\textbf{Model losses.}
Instead of using the actual losses, we compute model confidences as $\phi(f(\bx),\mathbf{y}) = \log (f(\bx)_y) - \log( \sum_{y'} f(\bx)_{y'})$. 
This score compares the confidence the model assigns to the true class (e.g., `positive') with the confidences the model assigns to all other classes (i.e., all other words from the approximately 250680 dimensional vocabulary). 
The higher the score is the more confident the model is in the correct prediction.
